# Supplementary material for: Compressing Neural Networks with the Hashing Trick
Source: arXiv:1504.04788 source file (2015-04-19)
Supplement: Supplementary file 1 [file appendix.tex]

%!TEX root=../hashnn_main.tex

\section*{Appendix}

In this section, Given a full-size neural network, we want to figure out how we can construct a smaller size of standard neural network that has the same size as the hashed full-size network.

Denote $n^l$ is the number of units in layer $l$ in full-size neural network and suppose there are $L$ layers. Denote $c$ as the compression factor where $0\leq c\leq 1$ is the compression factor. Note that we always don't the biases of last layer. The size of hashed neural network is as follows:
\begin{equation}
	N_{hash} = c \sum_{l=1}^{L-2} (n^l+1)n^{l+1} + c n^{L-1}n^L+n^L
\end{equation}
Suppose for smaller standard network, the number of units is $m^l=rn^l$ for $l=2,\cdots,L-1$ and $m^1=n^1, n^L=n^L$ because we don't shrink the input and output layer and the shrinkage factor is always $r$ for all hidden layers. The size of standard network is 
\begin{equation}
	\begin{aligned}
	&N_{standard} \\
	&= (m^1+1)m^2 + \sum_{l=2}^{L-2} (m^l+1)m^{l+1} +  m^{L-1}m^L+m^L \\
	&= (n^1+1)rn^2 + \sum_{l=2}^{L-2} (rn^l+1)rn^{l+1} + rn^{L-1}n^L+n^L \\
	&= r^2 \sum_{l=2}^{L-2}n^ln^{l+1} + r(\sum_{l=1}^{L-2} n^{l+1} + n^1n^2+n^{L-1}n^L)+n^L
	\end{aligned}
\end{equation}
Making $N_{standard}=N_{hash}$, we get
\begin{equation}
	\begin{aligned}
	&r^2 \sum_{l=2}^{L-2}n^ln^{l+1} + r\left(\sum_{l=1}^{L-2} n^{l+1} + n^1n^2+n^{L-1}n^L\right) \\
	&- c \left( \sum_{l=1}^{L-2} (n^l+1)n^{l+1} + n^{L-1}n^L \right) = 0
	\label{eq.quadratic}
	\end{aligned}
\end{equation}
Solving the above equation could get us the shrinkage factor $r$. The followings are some special cases:
\begin{enumerate}

	\item In the case of more than 3-layer network ($L\geq 3$), If we have the same amount of units in each hidden layer, \emph{i.e.} $n^2=\cdots=n^{L-1}=m$, Eq. \eqref{eq.quadratic} becomes
	\begin{equation}
		\begin{aligned}
		&r^2 (L-3)m^2 + r (L-2+n^1+n^L)m  \\
		&- c\left( (L-3)(m^2+m) + m(n^1 + n^L + 1)  \right)=0
		\end{aligned}
	\end{equation}
	
	\item In the case of 3-layer network ($L=3$), the quadratic term disappears which results in $r=c$.
	\item When $c>1$, $c$ stands for expansion factor. In other words, the virtual network is a large one, but the actual storage is still the same.
\end{enumerate}
